# Supplementary material for: Measurement of CP asymmetry in $B^0_s \rightarrow D^{\mp}_s K^{\pm}$ decays
Source: arXiv:1407.6127 source file (2014-11-26)
Supplement: Supplementary file 1 [file supplementary.pdf]

# 1 Supplementary material for LHCb-PAPER-2014-038

This short document contains supplementary material that will posted on the public cds record but will not appear in the paper.

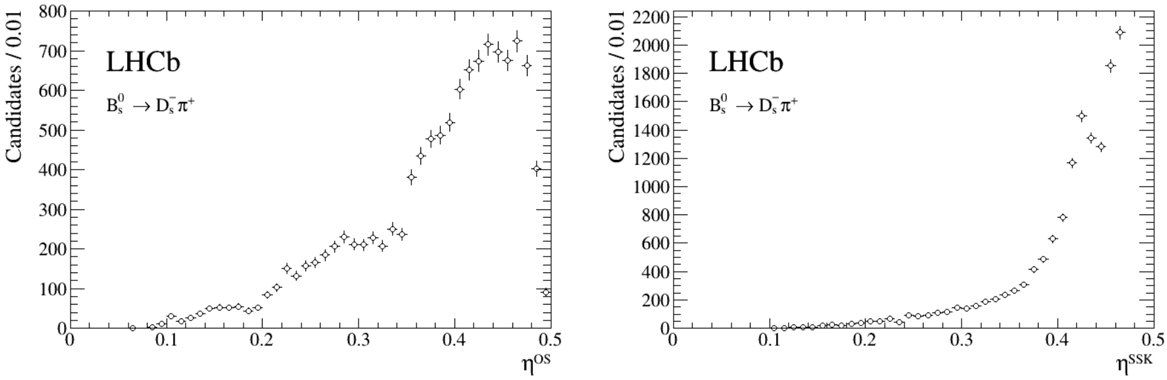


Figure 1: Mistag distributions for the uncalibrated output of the (left) opposite side and (right) same side Kaon tagger for the $B_s^0 \to D_s^- \pi^+$ control channel.

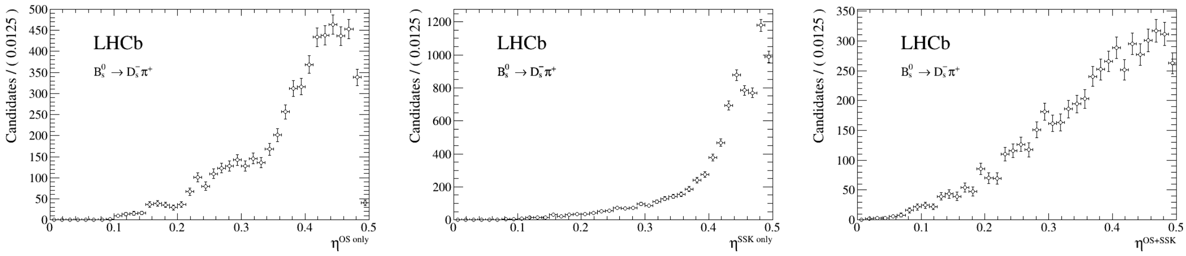


Figure 2: Mistag distributions for the calibrated output of the combination of opposite and same side Kaon taggers. The candidates from the $B_s^0 \to D_s^- \pi^+$ control channel have been split into candidates tagged by (left) only the opposite side tagger, (middle) only the same side Kaon tagger and (right) both taggers. As expected, the calibration does not change the shape of the distributions for candidates tagged by a single tagger only (*cf.* Fig. 8 in the paper). However, the distribution for candidates tagged by both taggers shows a marked increase at low mistag probabilities $\eta$ compared to the singly tagged ones as one would expect.

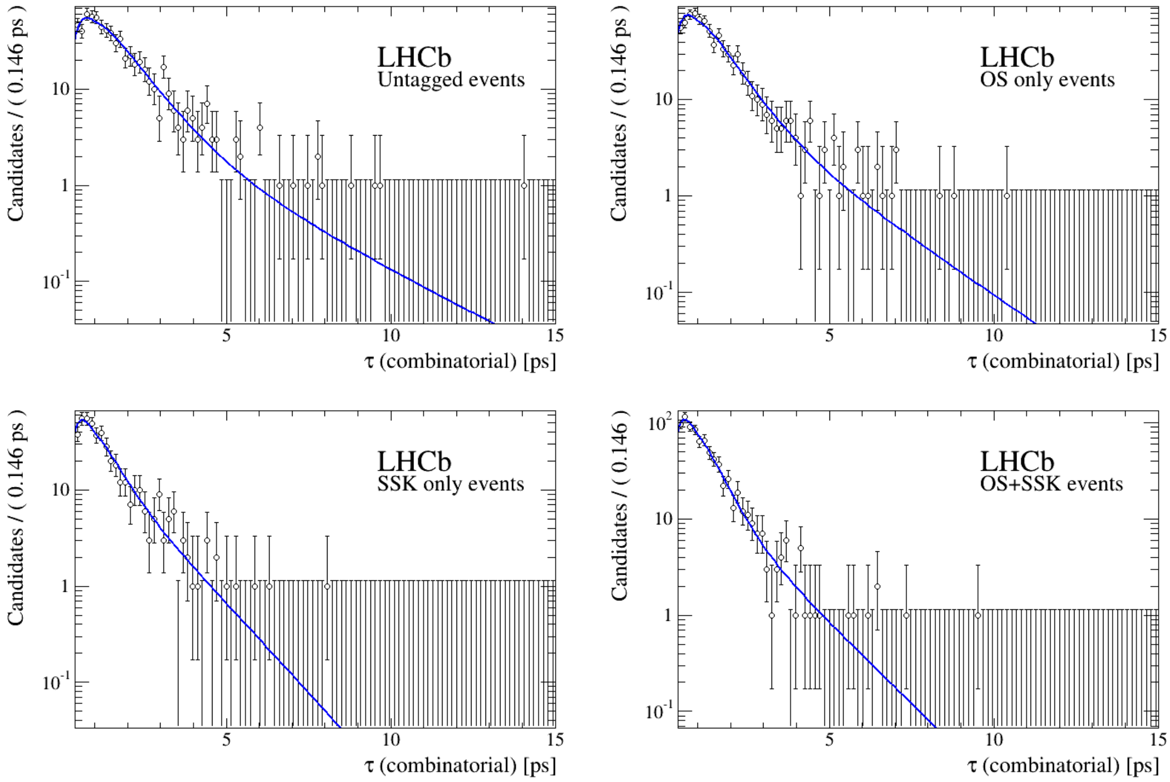


Figure 3: A fit to the high $B_s^0$ mass sideband ($5700\,\mathrm{GeV}/c^2 < m_{B_s} < 10\,000\,\mathrm{GeV}/c^2$) is used to extract the shapes of the combinatorial background as a function of decay time in the $B_s^0 \to D_s^{\mp} K^{\pm}$ analysis. All selection cuts have been applied. It is necessary to split the data into (top left) untagged, (top right) opposite side only, (bottom left) same side Kaon only candidates, and (bottom right) candidates tagged by both taggers. Physical backgrounds all have their characteristic momentum spectra due to the underlying hard scatter, and the tagging efficiencies vary slowly enough over the occurring momentum range that this effect can be treated. Combinatorial background spans a much wider range of momenta, which causes different apparent lifetimes for the four categories of candidates. The fit shows a double exponential model, convoluted with the per-event resolution function used in the analysis, and corrected for acceptance effects.

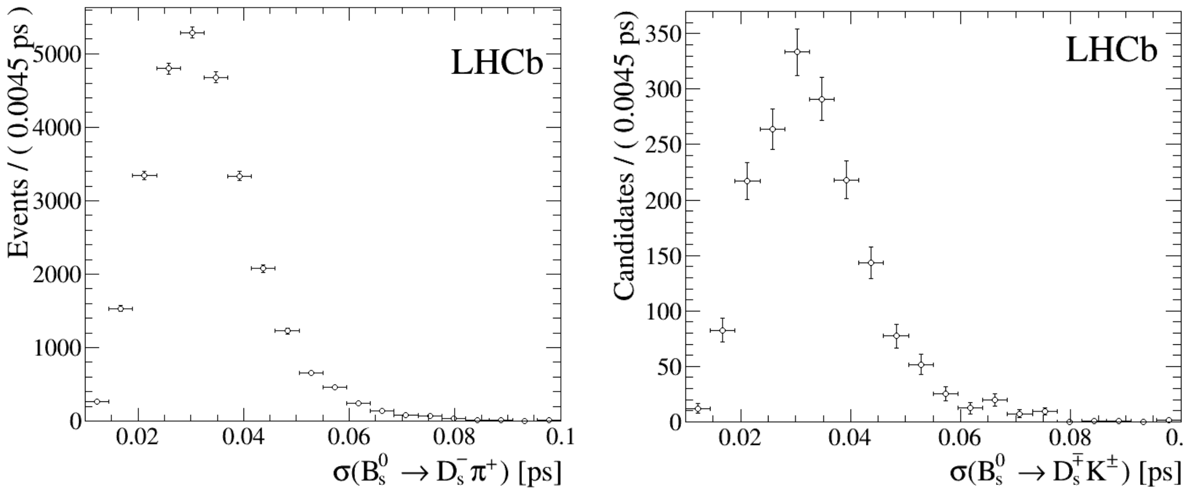


Figure 4: Estimated decay time error distributions provided by the decay time fit for (left) $B_s^0 \to D_s^- \pi^+$ and (right) $B_s^0 \to D_s^\mp K^\pm$ candidates. As explained previously, these have to be scaled up by a factor of $S = 1.37 \pm 0.10$ to obtain the true decay time (see Section 7 in the paper).

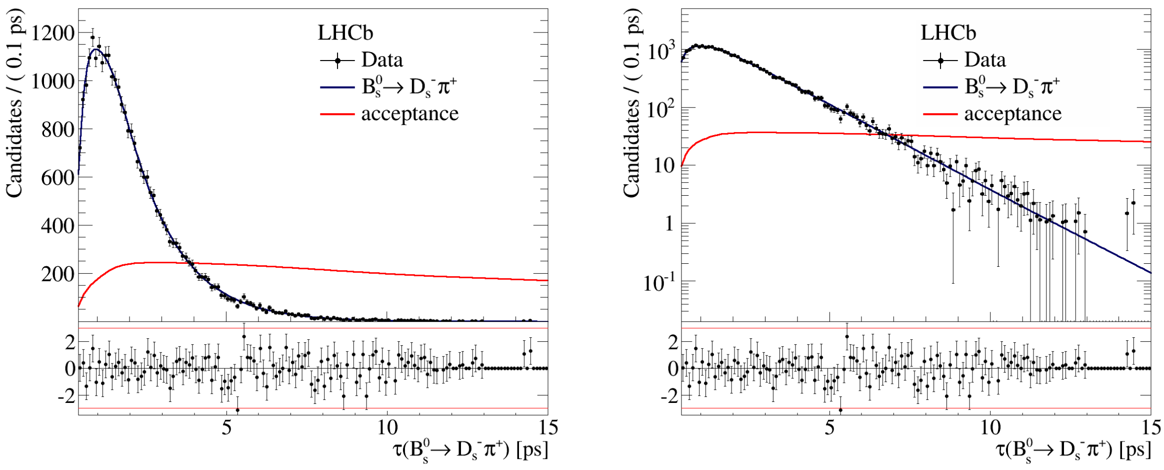


Figure 5: The decay time distribution of $B_s^0 \to D_s^- \pi^+$ candidates is used to determine the acceptance function in data. The left plot contains a time projection of the *sFit* result in linear scale, the right one shows the same in logarithmic scale (identical to Fig. 5 in the paper).

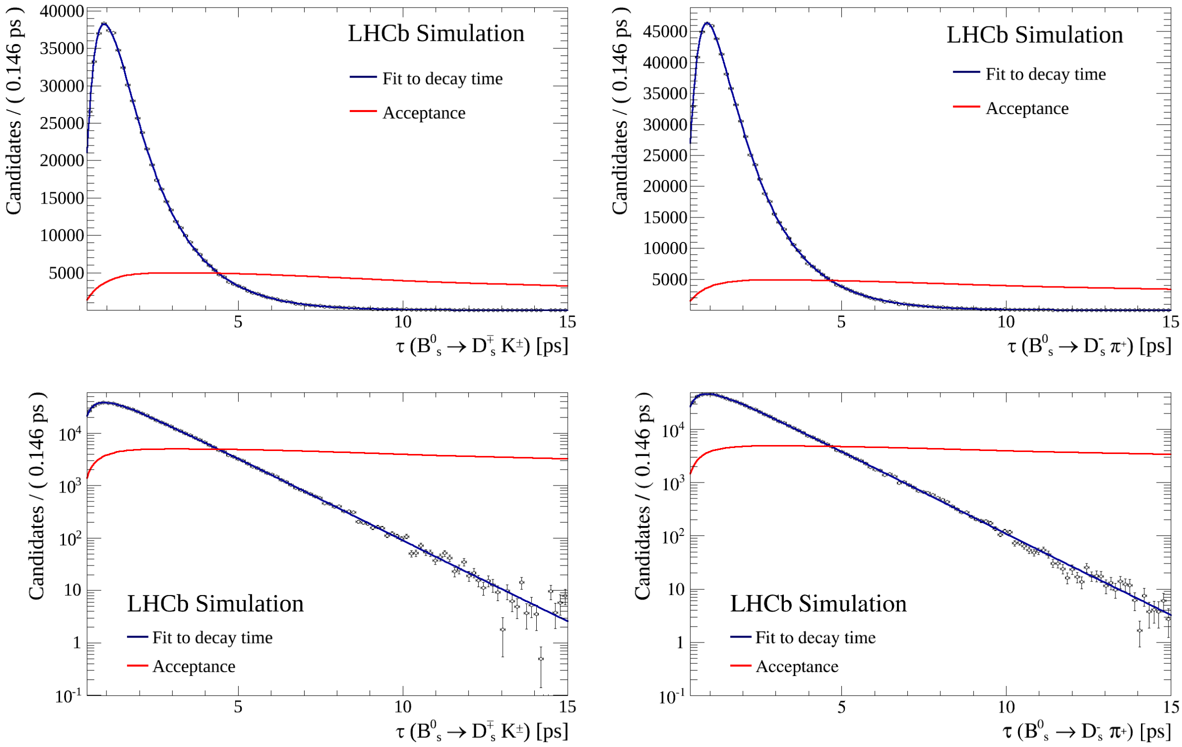


Figure 6: To obtain the $B_s^0 \to D_s^{\mp}K^{\pm}$ acceptance in data, the $B_s^0 \to D_s^-\pi^+$ acceptance as determined on data (*cf.* Fig. 5) is corrected with the ratio of (left) $B_s^0 \to D_s^{\mp}K^{\pm}$ over (right) $B_s^0 \to D_s^-\pi^+$ acceptances in simulated events. The top row shows the fits to simulated samples in linear scale to better show acceptance variations, the bottom row shows the excellent agreement in the tails in logarithmic scale. The acceptance functions are modelled with cubic splines with six knots (see Section 7 in the paper for details.)

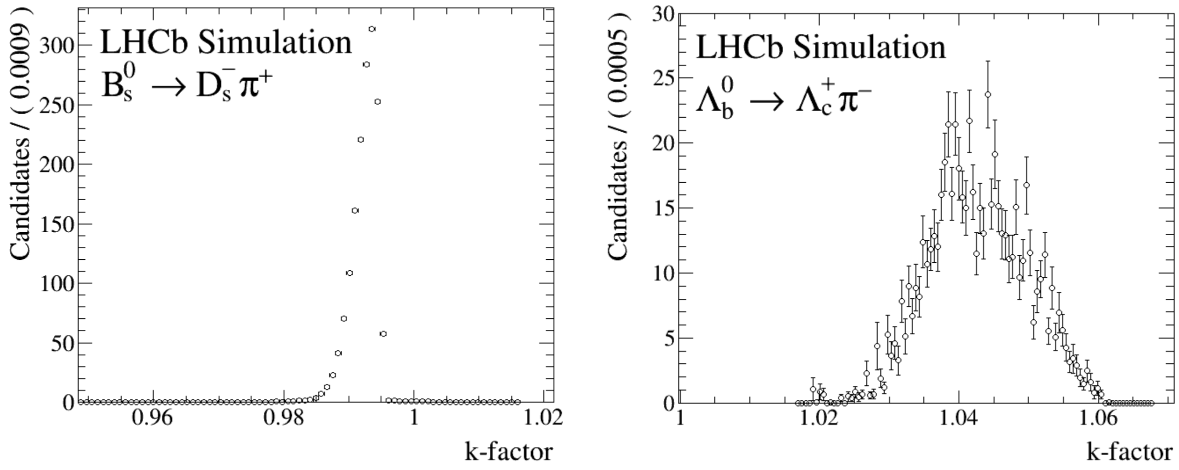


Figure 7: For partially reconstructed and misidentified modes, the reconstructed decay time is biased due to the loss of a particle or a wrong mass hypothesis. This can be corrected with the $k$-factor formalism by using simulated events to model the bias. The $k$-factor is defined as $k \equiv \frac{(m/p)_{\text{true}}}{(m/p)_{\text{reconstructed}}}$ where $p$ is the true (or reconstructed) $B$ meson momentum $p$ and $m$ its mass. The distribution of $k$ can be used to correct for these biases on a statistical basis. As an example, the plots show the $k$-factor distributions in simulated events for (left) $B_s^0 \to D_s^- \pi^+$ and (right) $\overline{\Lambda}_b^0 \to \overline{\Lambda}_c^- \pi^+$ candidates when reconstructed under the $B_s^0 \to D_s^\mp K^\pm$ mass hypothesis.

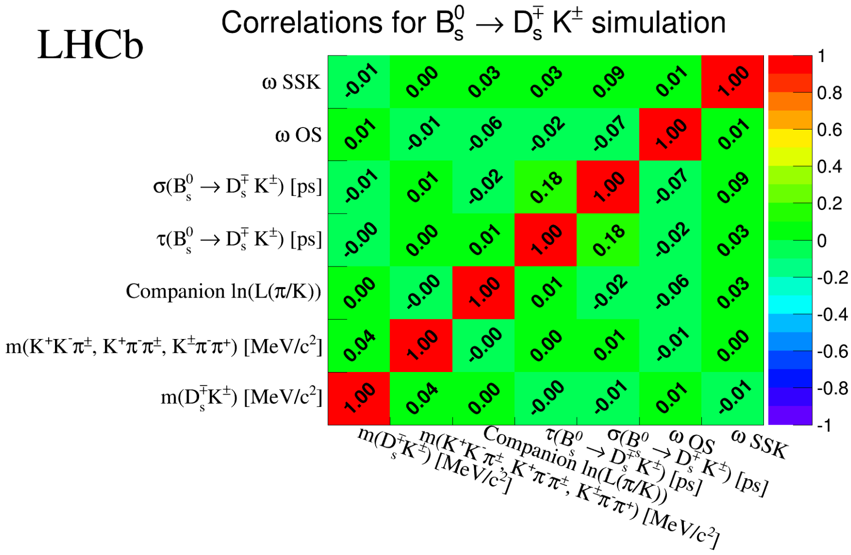


Figure 8: Linear correlation coefficients between the seven observables used in the analysis ($B_s^0$ mass, $D_s$ mass, companion PID log-likelihood difference, decay time, decay time error, and mistag rates for opposite side (OS) and same side Kaon (SSK) taggers) for $B_s^0 \to D_s^\mp K^\pm$ signal candidates from simulated events, given in percent. The correlations are small.

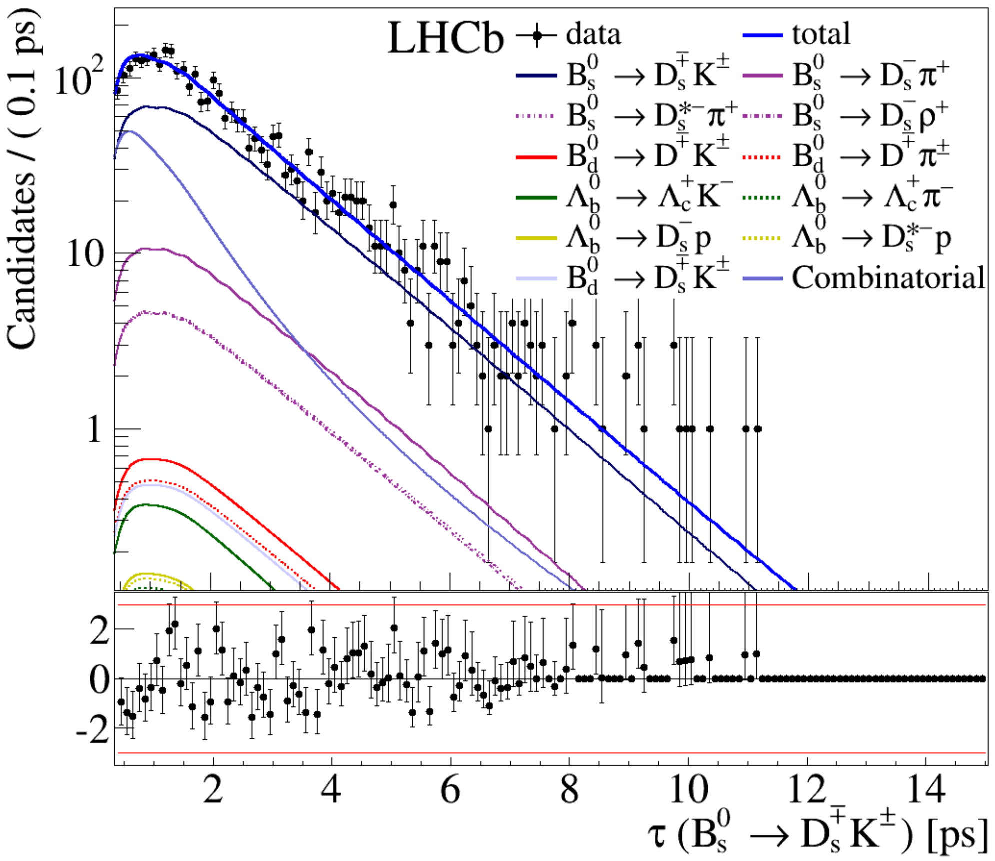


Figure 9: Result of the decay-time fit (*cFit*) to the $B_s^0 \to D_s^{\mp} K^{\pm}$ candidates; in contrast to Fig. 6 in the paper, the different background modes have not been merged into groups, and are displayed separately.
